# Supplementary material for: Towards Unified Benchmark and Models for Multi-Modal Perceptual Metrics
Source: arXiv:2412.10594 source file (2024-12-13)
Supplement: Supplementary file 1 [file X_suppl.tex]

\clearpage
\setcounter{page}{1}
\maketitlesupplementary

\section{Rationale}
\label{sec:rationale}
